# Supplementary material for: Multiplicity for a Group Sequential Trial with Biomarker Subpopulations
Source: arXiv:2004.08458 source file (2020-08-06)
Supplement: Supplementary file 1 [file CCT_Supplemental_file_V8__clean_.pdf]

**Supplemental file.**

## Appendix A – Derivation of Formula [2] for special case.

In this section, we will show the derivation of Formula [2].

Let $S_{i,k}$ be the logrank score statistic at analysis $k$ for population $i$ which follows the normal distribution asymptotically (Schoenfeld, 1981; Tsiatis, 1982) with

$$E[S_{i,k}] = -\ln(HR) \times n_{i,k} \times r(1-r)$$

$$Var[S_{i,k}] = n_{i,k} \times r(1-r)$$

where r is the proportion randomization to the experimental group. Under the null hypothesis, where HR=1, we have $-\ln(HR) = 0$. Therefore, $E[S_{i,k}] = 0$ and $Cov[S_{i,k}, S_{i',k'}] = E[S_{i,k}S_{i',k'}]$.

1) For $i = i'$, the Formula [2] is a standard group sequential design result for a single population and a time-to-event endpoint.
2) For $k = k'$, the Formula [2] is the result from Spiessens and DeBois (Spiessens & Debois, 2010) and Holmgren (Holmgren, 2017) since we are adding observations from an independent incremental subgroup and the covariance for the inclusive between the two populations is the variance of the smaller population.
3) For $i < i'$ and $k < k'$, $E[(S_{i',k'} - S_{i,k}) \times S_{i,k}] = E[S_{i',k'} - S_{i,k}] \times E[S_{i,k}] = 0$ using the independent increment property and $E[S_{i,k}S_{i',k'}] = E[S_{i,k}S_{i,k}] = D_{i,k} \times r(1-r)$ resulting in

$$Corr(S_{i,k}, S_{i',k'}) = \frac{Cov[S_{i,k}, S_{i',k'}]}{\sqrt{var(S_{i',k'})var(S_{i,k})}} = \frac{n_{i,k}}{\sqrt{n_{i',k'}n_{i,k}}}$$

4) For $i < i'$ and $k > k'$, we have

$$Cov(S_{i,k}, S_{i',k'}) = E[(S_{i,k'} + (S_{i,k} - S_{i,k'}))(S_{i,k'} + (S_{i',k'} - S_{i,k'}))] = Var[S_{i,k'}]$$

since increments are independent in between both nested populations and analyses leading to other terms dropping out. This then leads to

$$Corr(S_{i,k}, S_{i',k'}) = \frac{Cov[S_{i,k}, S_{i',k'}]}{\sqrt{var(S_{i',k'})var(S_{i,k})}} = \frac{n_{i,k'}}{\sqrt{n_{i',k'}n_{i,k}}}$$

## Appendix B – Alternative algorithms to compute testing bounds

In Section 3.2.1, we described Algorithm 1 to compute the testing bounds. Here we describe Algorithm 2 and Algorithm 3 as alternatives.

Define $\alpha_k(J)$ as the cumulative alpha spent up to analysis $k$ for an intersection hypothesis $H_J, J \subseteq I$

$$\alpha_k(J) = \sum_{i \in J} f_i(t_{ik};\ w_i(J) \times \alpha)$$

**Algorithm 2:**

For a given $J \subseteq I$ and sequentially for analysis $k \in 1, \dots, K$:

1. Assume for $j < k$ that bounds $b_{ij} = c_{ij}(J), j < k, i \in J$, have already been set.
2. Based on the $n_{ik}$ at analysis $k$, compute the bounds $b_{ik}$.
   a. Choose a nominal $\alpha_k^*(J) > \alpha_k(J) - \alpha_{k-1}(J)$
   b. $b_{ik} = \Phi(1 - w_i(J)\alpha_k^*(J))$
   c. Compute type I error rate up to analysis $k$ as described in equation (4) of Section 3.2. That is,
   $$1 - \Pr\left( \bigcap_{i \in J} \{Z_{ik} < b_{ik}\} \bigcap_{1 \leq j < k} \{Z_{ij} < c_{ij}(J)\} | H_J \right)$$
   d. Update $\alpha_k^*(J)$ until this type I error rate up to analysis $k$ is controlled at $\alpha_k(J)$ for $H_J$. That is,
   $$1 - \Pr\left( \bigcap_{i \in J} \{ Z_{ik} < b_{ik}\} \bigcap_{1 \leq j < k} \{Z_{ij} < c_{ij}(J)\} | H_J \right) = \alpha_k(J)$$
   e. After the appropriate $\alpha_k^*(J)$ has been derived, $b_{ik}$ is computed as in step b, and then we set $c_{ik}(J) = b_{ik}$.

**Algorithm 3:**

For nested populations, in intersection hypothesis $H_J$, define the index of the largest population as $m$. In this approach, the boundaries for the non-largest populations are kept as the boundaries from the Bonferroni approach without accounting for population correlation, and only to adjust the boundaries for the largest population $M$ when population correlation is incorporated.

For a given $J \subseteq I$ and sequentially for analysis $k \in 1, \dots, K$:

1. Assume for $j < k$ that bounds $b_{ij} = c_{ij}(J), j < k, i \in J$, have already been set.
2. Based on the $n_{ik}$ at analysis $k$, compute the bounds $b_{ik}$.

a. For $i \neq m$, $b_{ik}$ are such that

$$1 - \Pr\left( \{Z_{ik} < b_{ik}\} \bigcap_{1 \leq j < k} \{Z_{ij} < c_{ij}(J)\} | H_{i0} \right) = f_i(t_{ik};\ w_i(J) \times \alpha)$$

b. Once the $b_{ik}$ are computed for $i \neq m$, $b_{mk}$ is such that

$$1 - \Pr\left( \bigcap_{i \in J} \{Z_{mk} < b_{mk}\} \bigcap_{1 \leq j < k} \{Z_{ij} < c_{ij}(J)\} \bigcap_{i \neq m} \{Z_{ik} < b_{ik}\} | H_0 \right) = \alpha_k(J)$$

c. Set $c_{ik}(J) = b_{ik}$ for all $i \in J$.

## Appendix C - R program example in Section 4

### Introduction

Below is an example of R program for application of Complete Correlation Structure (CCS) based on the same setting as in the Section 4. We assume i.i.d. observations in a 2-arm trial testing for treatment effect in a subgroup and overall population. Suppose one interim analysis will be performed at 50% pending time of the trial and the prevalence of the subgroup is also 50%. The correlation matrix for the interim test statistics $Z_{11}$, $Z_{12}$ and final test statistics $Z_{21}$, $Z_{22}$ is

$$\begin{bmatrix} 1 & \sqrt{0.5} & \sqrt{0.5} & 0.5 \\ \sqrt{0.5} & 1 & 0.5 & \sqrt{0.5} \\ \sqrt{0.5} & 0.5 & 1 & \sqrt{0.5} \\ 0.5 & \sqrt{0.5} & \sqrt{0.5} & 1 \end{bmatrix}$$

### Nominal Alpha Allocation

We set up a group sequential design using Lan-DeMets spending function to approximate O'Brien-Fleming bound for both subgroup and the overall population and equaly split Type I error of 2.5% (1-sided) into two populations. The boundaries for Z-statistics in interim and final naalysis can be calculated as below.

### Design setup

```
# Clean out data
rm(list=ls())

# Loading packages
library(xtable)
library(ggplot2)
library(gsDesign)
library(mvtnorm)

# Regular GS design bounds
z <- gsDesign(test.type=1,k=2,sfu=sfLDOF,alpha=.0125)$upper$bound
round(z,3)

## [1] 3.345 2.246

# Construct correlation matrix
corrmatrix <- matrix(.5^c( 0,.5,.5, 1,
                    .5, 0, 1,.5,
                    .5, 1, 0,.5,
                    1,.5,.5, 0),nrow=4)
corrmatrix

##          [,1]      [,2]      [,3]      [,4]
## [1,] 1.0000000 0.7071068 0.7071068 0.5000000
## [2,] 0.7071068 1.0000000 0.5000000 0.7071068
```

```
## [3,] 0.7071068 0.5000000 1.0000000 0.7071068
## [4,] 0.5000000 0.7071068 0.7071068 1.0000000
```

The overall 1-sided Type I error with above correlation structure can be calculated using $pmvnorm$ function

```
# Study familywise Type I error and compared to 0.025
tru_stu_alpha <- 1-pmvnorm(upper=c(z[1],z[1],z[2],z[2]),corr=cormatrix, algorithm = Miwa())[1]
round(tru_stu_alpha,4)

## [1] 0.0214
```

As compared to the setting of family-wise error rate 0.025, we only use 0.0214 nominal alpha level in the study.

Next, we build a function to compute the adjusted nominal alpha level.

```
nomalpha <- function(x,target,cormatrix){
  z <- gsDesign(test.type=1,k=2,sfu=sfLDOF,
              alpha=x)$upper$bound
  return(1-pmvnorm(upper=c(z[1],z[1],z[2],z[2]),
                corr=cormatrix, algorithm = Miwa())[1]-target)
}
# adjusted nominal alpha
alphaadj <- uniroot(nomalpha,lower=.0125,upper=.025,
                   target=.025,cormatrix=cormatrix)$root
round(alphaadj,4)

## [1] 0.0147

# alternative bounds
altbound <- gsDesign(k=2,test.type=1,alpha=alphaadj,
                    sfu=sfLDOF)$upper$bound
round(altbound,3)

## [1] 3.260 2.184
```

The alternative boundaries are 3.26, 2.184 with respect to adjusted nominal alpha level 0.0147. Compared to regular group sequential design boundaries, 3.345, 2.246, CCS-adjusted group sequential design has ease boundaries.

**Population power**

We set up the effect size at 0.15 and chose a portion of $1/\sqrt{2}$ to obtain the same power in each population.

```
# Effect size
delta <- 0.15/c(1,sqrt(2))
x1 <- gsDesign(delta=delta[1],k=2,sfu=sfLDOF,alpha=.0125)
x2 <- gsDesign(delta=delta[2],k=2,sfu=sfLDOF,alpha=.0125)

# Subgroup power
```

```
power.sub <- sum(gsProbability(theta=delta[1],n.I=ceiling(x1$n.I),
              k=2,a=c(-20,-20),b=altbound)$upper$prob)
# Overall power
power.ova <- sum(gsProbability(theta=delta[2],n.I=ceiling(x2$n.I),
              k=2,a=c(-20,-20),b=altbound)$upper$prob)
round(power.sub,3)

## [1] 0.919

round(power.ova,3)

## [1] 0.919
```

The population power adjusted with CCS in group sequential design is 0.919. It elevates about 2% from default power setting at 0.9.

**Sample size**

The sample size in regular group sequential design is calculated as below.

```
N <- ceiling(c(x1$n.I[2],x2$n.I[2]))
N

## [1]  570 1140
```

570 subjects in subgroup and 1140 subjects in overall population.

The CCS-adjusted sample size with fixed power (0.9) and fixed effect size are calculated as below.

```
# Subgroup
SS.sub <- ceiling(gsDesign(k=2,sfu=sfLDOF,delta=delta[1],alpha=alphaadj)$n.I[2])
SS.sub

## [1] 551

# Overall
SS.ova <- ceiling(gsDesign(k=2,sfu=sfLDOF,delta=delta[2],alpha=alphaadj)$n.I[2])
SS.ova

## [1] 1101
```

The required sample sizes are 551 in subgroup and 1101 in the overall population. We save 19 subjects and 39 subjects in the subgroup and overall population respectively.

**Appendix D - R program in Section 5**

```
# Clean out data
rm(list=ls())
# loading packages
library(xtable)
library(ggplot2)
library(gsDesign)
library(mvtnorm)
z1 <- gsSurv ( k = 3 , test.type = 4 , alpha = 0.0125 , beta = 0.1,
        timing = c( 0.5,0.75 ) , sfu = sfLDOF , sfupar = c( 0 ) ,
        sfl = sfHSD , sflpar = c( -8 ) , lambdaC = log(2) / 17.5 ,
        hr = 0.65 , hr0 = 1 , eta = 0.0025 , gamma = c( 2.5,5,7.5,10 ) ,
        R = c(1,1,1,8 ) ,S = NULL , T = 37.5 , minfup = 26.5 , ratio = 2)$upper$bound
z2 <- gsSurv ( k = 3 , test.type = 4 , alpha = 0.0125 , beta = 0.1,
        timing = c( 0.5,0.75 ) , sfu = sfLDOF , sfupar = c( 0 ) ,
        sfl = sfHSD , sflpar = c( -8 ) , lambdaC = log(2) / 17.5 ,
        hr = 0.7 , hr0 = 1 , eta = 0.0025 , gamma = c( 2.5,5,7.5,10 ) ,
        R = c(1,1,1,8 ),S = NULL , T = 37.5 , minfup = 26.5 , ratio = 2 )$upper$bound
round(z1,3)
```

```
## [1] 3.345 2.670 2.281
```

**CCS correlation matrix**

```
corr_6by6 <- function(p_s, t_i1, t_i2){
        # p_s is Proportion of subgroup
        # t_i1 is information time proportion of first IA
        # t_i2 is information time proportion of second IA
        # Covariance formula
        covZ <- function(p1,p2,t1,t2){
        sqrt((min(p1,p2)*min(t1,t2))/(max(p1,p2)*max(t1,t2)))
        }
        cov12 <- covZ(p_s,1,t_i1,t_i1)
        cov13 <- covZ(p_s,p_s,t_i1,t_i2)
        cov14 <- covZ(p_s,1,t_i1,t_i2)
        cov15 <- covZ(p_s,p_s,t_i1,1)
        cov16 <- covZ(p_s,1,t_i1,1)
        cov23 <- covZ(1,p_s,t_i1,t_i2)
        cov24 <- covZ(1,1,t_i1,t_i2)
        cov25 <- covZ(1,p_s,t_i1,1)
        cov26 <- covZ(1,1,t_i1,1)
        cov34 <- covZ(p_s,1,t_i2,t_i2)
        cov35 <- covZ(p_s,p_s,t_i2,1)
        cov36 <- covZ(p_s,1,t_i2,1)
```

```
        cov45 <- covZ(1,p_s,t_i2,1)
        cov46 <- covZ(1,1,t_i2,1)
        cov56 <- covZ(1,p_s,1,1)
        # build up corr matrix
        corrmatrix <- matrix(c(1, cov12, cov13, cov14, cov15, cov16,
        cov12, 1, cov23, cov24, cov25, cov26,
        cov13, cov23, 1, cov34, cov35, cov36,
        cov14, cov24, cov34, 1, cov45, cov46,
        cov15, cov25, cov35, cov45, 1, cov56,
        cov16, cov26, cov36, cov46, cov56, 1),nrow=6)
        corrmatrix
}
corrmatrix <- corr_6by6(p_s=0.6, t_i1=0.5, t_i2=0.75)
```

**Adjusted nominal Alpha Level**

```
nomalpha <- function(x,target,corrmatrix){
z1 <- gsSurv ( k = 3 , test.type = 4 , alpha = x , beta = 0.1,
        timing = c( 0.5,0.75 ) , sfu = sfLDOF , sfupar = c( 0 ) ,
        sfl = sfHSD , sflpar = c( -8 ) , lambdaC = log(2) / 17.5 ,
        hr = 0.65 , hr0 = 1 , eta = 0.0025 , gamma = c( 2.5,5,7.5,10 ) ,
        R = c(1,1,1,8 ) ,S = NULL , T = 37.5 , minfup = 26.5 , ratio = 2)$upper$bound
z2 <- gsSurv ( k = 3 , test.type = 4 , alpha = x , beta = 0.1,
        timing = c( 0.5,0.75 ) , sfu = sfLDOF , sfupar = c( 0 ) ,
        sfl = sfHSD , sflpar = c( -8 ) , lambdaC = log(2) / 17.5 ,
        hr = 0.7 , hr0 = 1 , eta = 0.0025 , gamma = c( 2.5,5,7.5,10 ) ,
        R = c(1,1,1,8 ),S = NULL , T = 37.5 , minfup = 26.5 , ratio = 2 )$upper$bound
return(1-pmvnorm(upper=c(z1[1],z2[1],z1[2],z2[2],z1[3],z2[3]),
corr=corrmatrix, algorithm = Miwa())[1]-target)}
alphaadj <- uniroot(nomalpha,lower=.010,upper=.025,
target=.025,corrmatrix=corrmatrix)$root
alphaadj
```

```
## [1] 0.01532291
```

```
altbound <- gsSurv ( k = 3 , test.type = 4 , alpha = alphaadj , beta = 0.1,
        timing = c( 0.5,0.75 ) , sfu = sfLDOF , sfupar = c( 0 ) ,
        sfl = sfHSD , sflpar = c( -8 ) , lambdaC = log(2) / 17.5 ,
        hr = 0.7 , hr0 = 1 , eta = 0.0025 , gamma = c( 2.5,5,7.5,10 ) ,
        R = c(1,1,1,8 ),S = NULL , T = 37.5 , minfup = 26.5 , ratio = 2 )$upper$bound
round(altbound,2)
```

```
## [1] 3.24 2.58 2.21
```

**Sample Size using Bonferroni-adjusted GS design**

```
#Subgroup
x1 <- gsSurv ( k = 3 , test.type = 4 , alpha = 0.0125 , beta = 0.1,
        timing = c( 0.5,0.75 ) , sfu = sfLDOF , sfupar = c( 0 ) ,
        sfl = sfHSD , sflpar = c( -8 ) , lambdaC = log(2) / 17.5 ,
        hr = 0.65 , hr0 = 1 , eta = 0.0025 , gamma = c( 2.5,5,7.5,10 ) ,
        R = c(1,1,1,8 ) ,S = NULL , T = 37.5 , minfup = 26.5 , ratio = 2)
#Overall
x2 <- gsSurv ( k = 3 , test.type = 4 , alpha = 0.0125 , beta = 0.1,
        timing = c( 0.5,0.75 ) , sfu = sfLDOF , sfupar = c( 0 ) ,
        sfl = sfHSD , sflpar = c( -8 ) , lambdaC = log(2) / 17.5 ,
        hr = 0.7 , hr0 = 1 , eta = 0.0025 , gamma = c( 2.5,5,7.5,10 ) ,
        R = c(1,1,1,8 ),S = NULL , T = 37.5 , minfup = 26.5 , ratio = 2 )
N2 <- ceiling(c(x1$n.I[3], x2$n.I[3]))
N2
## [1] 296 434
```

**Sample Size using CCS GS design**

```
N_sub <- ceiling(gsSurv ( k = 3 , test.type = 4 , alpha = alphaadj , beta = 0.1,
        timing = c( 0.5,0.75 ) , sfu = sfLDOF , sfupar = c( 0 ) ,
        sfl = sfHSD , sflpar = c( -8 ) , lambdaC = log(2) / 17.5 ,
        hr = 0.65 , hr0 = 1 , eta = 0.0025 , gamma = c( 2.5,5,7.5,10 ) ,
        R = c(1,1,1,8 ) ,S = NULL , T = 37.5 , minfup = 26.5 , ratio = 2)$n.I[3])
N_Overall <- ceiling(gsSurv ( k = 3 , test.type = 4 , alpha = alphaadj , beta = 0.1,
        timing = c( 0.5,0.75 ) , sfu = sfLDOF , sfupar = c( 0 ) ,
        sfl = sfHSD , sflpar = c( -8 ) , lambdaC = log(2) / 17.5 ,
        hr = 0.7 , hr0 = 1 , eta = 0.0025 , gamma = c( 2.5,5,7.5,10 ) ,
        R = c(1,1,1,8 ),S = NULL , T = 37.5 , minfup = 26.5 , ratio = 2 )$n.I[3])
N_corr_adjusted <- c(N_sub, N_Overall)
N_corr_adjusted
## [1] 283 415
```

**Power**

```
power.subgroup <- sum(gsProbability(theta=x1$delta, n.I=ceiling(x1$n.I),k=3,
        a=c(-20,-20,-20), b=altbound)$upper$prob)
power.overall <- sum(gsProbability(theta=x2$delta, n.I=ceiling(x2$n.I),k=3,
        a=c(-20,-20,-20), b=altbound)$upper$prob)
power.subgroup
## [1] 0.9139928
```

### HR bound using Bonferroni-adjusted GS design

```
IA1.HR.bound <- exp(-3.35/sqrt(217*(1/3)*(2/3)))
IA2.HR.bound <- exp(-2.67/sqrt(326*(1/3)*(2/3)))
FA.HR.bound <- exp(-2.28/sqrt(434*(1/3)*(2/3)))
a_HR_e <- round(c(IA1.HR.bound, IA2.HR.bound, FA.HR.bound),2)
a_HR_e
## [1] 0.62 0.73 0.79
```

### HR bound using CCS GS design

```
IA1.HR.bound_a <- exp(-3.24/sqrt(217*(1/3)*(2/3)))
IA2.HR.bound_a <- exp(-2.58/sqrt(326*(1/3)*(2/3)))
FA.HR.bound_a <- exp(-2.21/sqrt(434*(1/3)*(2/3)))
a_HR_a <- round(c(IA1.HR.bound_a, IA2.HR.bound_a, FA.HR.bound_a),2)
a_HR_a
## [1] 0.63 0.74 0.80
```

### Reference


Holmgren, E. (2017). The application of group sequential stopping boundaries to evaluate the treatment effect of an experimental agent across a range of biomarker expression. *Contemp Clin Trials, 63*, 13-18. doi:10.1016/j.cct.2017.02.006

Schoenfeld, D. (1981). The asymptotic properties of nonparametric tests for comparing survival distributions. *Biometrika, 68*(1), 316-319.

Spiessens, B., & Debois, M. (2010). Adjusted significance levels for subgroup analyses in clinical trials. *Contemp Clin Trials, 31*(6), 647-656. doi:10.1016/j.cct.2010.08.011

Tsiatis, A. A. (1982). Repeated significance testing for a general class of statistics used in censored survival analysis. *Journal of the American Statistical Association, 77*(380), 855-861.
